# Supplementary material for: A Principled Framework for Knowledge-enhanced Large Language Model
Source: arXiv:2311.11135 source file (2023-11-18)
Supplement: Supplementary file 1 [file appendix.tex]

\section{You \emph{can} have an appendix here.}

You can have as much text here as you want. The main body must be at most $8$ pages long.
For the final version, one more page can be added.
If you want, you can use an appendix like this one, even using the one-column format.
